# Supplementary material for: C-SHORe: Higher-Order Verification via Collapsible Pushdown System Saturation
Source: arXiv:1703.04429 source file (2018-09-17)
Supplement: Supplementary file 1 [file appendix.tex]

\section{Full Experimental Results}
\label{sec:experiments-appendix}

The full experimental results are given below.
In the main paper we restricted attention to trials where at least one tool took over 1s.
This is because virtual machine ``warm-up'' and HORS to CPDS conversion can skew the results on small benchmarks.

We begin with a comparison of the different tools.

\begin{center}
    \small
    \begin{tabular}{lcccccccc}
        \toprule
        Benchmark file & Ord & Sz & T & TMC & G & C & P & H  \\
        \midrule
        \texttt{example2-1} & 1 & 7 & 0.003 & 0.031 & 0.011 & 0.050 & 0.259 & 0.003  \\
        \texttt{example2-3} & 1 & 13 & 0.002 & 0.030 & 0.010 & 0.045 & 0.264 & 0.003  \\
        \texttt{example3-1} (bug) & 1 & 8 & 0.000 & 0.102 & 0.009 & 0.057 & 0.256 & 0.003  \\
        \texttt{exception} & 1 & 18 & 0.002 & 0.029 & 0.010 & 0.045 & 0.262 & 0.003  \\
        \texttt{file} & 1 & 8 & 0.000 & 0.030 & 0.010 & 0.050 & 0.255 & 0.003  \\
        \texttt{fileocamlc} & 4 & 111 & 0.026 & 0.044 & 0.126 & 0.415 & 0.274 & 0.010  \\
        \texttt{filewrong} (bug) & 4 & 45 & 0.000 & 0.100 & 0.046 & 0.241 & 0.275 & 0.006  \\
        \texttt{flow} & 4 & 16 & 0.003 & 0.032 & 0.012 & 0.078 & 0.271 & 0.002  \\
        \texttt{lock1} & 4 & 38 & 0.010 & 0.034 & 0.019 & 0.091 & 0.267 & 0.003  \\
        \texttt{lock2} & 4 & 45 & 0.034 & 0.047 & 0.377 & 0.407 & 0.302 & 0.010  \\
        \texttt{order5} & 5 & 52 & 0.016 & 0.040 & --- & 0.431 & 0.267 & 0.009  \\
        \texttt{order5-2} & 5 & 40 & 0.048 & 0.063 & --- & 0.299 & 0.288 & 0.007  \\
        \texttt{order5-variant} & 5 & 55 & 0.042 & 0.040 & 1.663 & 0.464 & 0.297 & 0.010  \\
        \texttt{twofiles} & 4 & 47 & 0.017 & 0.038 & 0.169 & 0.260 & 0.291 & 0.006  \\
        \texttt{twofilesexn} & 4 & 56 & 0.020 & 0.037 & 0.090 & 0.254 & 0.288 & 0.008  \\
\\
        \texttt{checknz} & 2 & 93 & 0.010 & 0.034 & 0.020 & 0.077 & 0.296 & 0.003  \\
        \texttt{checkpairs} (bug) & 2 & 251 & 0.004 & 0.104 & 0.079 & 0.243 & 0.308 & 0.007  \\
        \texttt{filepath} & 2 & 5956 & 214.182 & --- & --- & 0.365 & 0.475 & 0.038  \\
        \texttt{filter-nonzero} (bug) & 5 & 484 & 0.013 & 0.133 & 0.282 & 1.532 & 0.529 & 0.026  \\
        \texttt{filter-nonzero-1} & 5 & 890 & 0.280 & 95.373 & --- & 5.129 & 1.914 & 0.098  \\
        \texttt{last} & 2 & 193 & 0.019 & 0.038 & 0.042 & 0.119 & 0.278 & 0.007  \\
        \texttt{map-head-filter} (bug) & 3 & 370 & 0.009 & 0.114 & 0.223 & 0.388 & 0.368 & 0.012  \\
        \texttt{map-head-filter-1} & 3 & 880 & 0.241 & 0.693 & --- & 0.391 & 0.340 & 0.016  \\
        \texttt{map-plusone} & 5 & 302 & 0.027 & 0.082 & 0.216 & 0.868 & 0.381 & 0.013  \\
        \texttt{map-plusone-1} & 5 & 459 & 0.047 & 0.375 & --- & 1.402 & 0.446 & 0.034  \\
        \texttt{map-plusone-2} & 5 & 704 & 1.429 & 6.125 & --- & 2.762 & 0.560 & 0.080  \\
        \texttt{mkgroundterm} & 2 & 379 & 0.090 & 0.062 & 0.093 & 0.219 & 0.290 & 0.007  \\
        \texttt{risers} & 2 & 563 & 0.111 & 0.070 & 0.120 & 0.348 & 0.382 & 0.009  \\
        \texttt{safe-head} & 3 & 354 & 0.047 & 0.048 & 0.117 & 0.365 & 0.337 & 0.011  \\
        \texttt{safe-init} & 3 & 680 & 0.066 & 0.136 & 0.404 & 0.661 & 0.376 & 0.013  \\
        \texttt{safe-tail} & 3 & 468 & 0.063 & 0.048 & 0.163 & 0.493 & 0.370 & 0.013  \\
        \texttt{tails} & 3 & 259 & 0.047 & 0.042 & 0.546 & 0.147 & 0.280 & 0.007  \\
\\
        \texttt{g41} & 4 & 31 & --- & 0.044 & 0.182 & --- & 0.300 & 0.007  \\
        \texttt{merge4} & 2 & 141 & 0.138 & 0.141 & 0.588 & 0.516 & 0.433 & 0.019  \\
        \texttt{stress} & 1 & 35 & 0.047 & 0.088 & 0.010 & 0.058 & 0.261 & 0.003  \\
\\
        \texttt{cfa-life2} & 14 & 7648 & --- & --- & --- & --- & 0.834 & 0.164  \\
        \texttt{cfa-matrix-1} & 8 & 2944 & 17.239 & --- & --- & 18.098 & 0.386 & 0.053  \\
        \texttt{cfa-psdes} & 7 & 1819 & 18.157 & --- & --- & 1.798 & 0.317 & 0.030  \\
        \texttt{dna} & 2 & 411 & 0.067 & 0.169 & 0.091 & 7.062 & 11.428 & 0.037  \\
        \texttt{exp4-5} & 4 & 55 & --- & --- & 0.939 & --- & 0.366 & 0.009  \\
        \texttt{fibstring} & 4 & 29 & --- & 33.039 & 0.189 & --- & 0.272 & 0.007  \\
        \texttt{filewrong} (bug) & 4 & 45 & 0.000 & 0.101 & 0.051 & 0.211 & 0.276 & 0.006  \\
        \texttt{fold\_fun\_list} & 7 & 1346 & 0.617 & --- & --- & 1.363 & 0.302 & 0.020  \\
        \texttt{fold\_right} & 5 & 1310 & 32.429 & --- & --- & 1.190 & 0.304 & 0.026  \\
        \texttt{jwig-cal\_main} & 2 & 7627 & 0.123 & 0.049 & 0.279 & 2.492 & 0.479 & 0.140  \\
        \texttt{l} & 3 & 35 & --- & 7.303 & 0.020 & 0.256 & 0.273 & 0.006  \\
        \texttt{search-e-church} (bug) & 6 & 837 & 0.023 & 0.206 & --- & 5.389 & 3.588 & 0.038  \\
        \texttt{specialize\_cps\_coerce1-c} & 3 & 2731 & --- & --- & --- & 0.950 & 0.409 & 0.188  \\
        \texttt{tak} (dunno) & 8 & 451 & --- & 1.980 & --- & 57.130 & 3.190 & 0.088  \\
        \texttt{xhtmlf-div-2} (bug) & 2 & 3003 & 0.327 & --- & 42.256 & 2.327 & 1.419 & 1.587  \\
        \texttt{xhtmlf-m-church} & 2 & 3027 & 0.304 & --- & 8.318 & 2.394 & 0.729 & 1.124  \\
        \texttt{zip} & 4 & 2952 & 22.771 & --- & --- & 2.808 & 0.713 & 0.059  \\

        \bottomrule
    \end{tabular}
\end{center}

Finally, we show a breakdown of the performance aspects of \cshore.

\begin{center}
    \small
    \begin{tabular}{lcccccc}
        \toprule
        Benchmark file & Ord & Sz & C & Ctran & Ccpds & Capprox  \\
        \midrule
        \texttt{example2-1} & 1 & 7 & 0.050 & 0.026 & 0.024 & 0.018  \\
        \texttt{example2-3} & 1 & 13 & 0.045 & 0.027 & 0.018 & 0.012  \\
        \texttt{example3-1} (bug) & 1 & 8 & 0.057 & 0.027 & 0.030 & 0.016  \\
        \texttt{exception} & 1 & 18 & 0.045 & 0.027 & 0.019 & 0.011  \\
        \texttt{file} & 1 & 8 & 0.050 & 0.027 & 0.023 & 0.017  \\
        \texttt{fileocamlc} & 4 & 111 & 0.415 & 0.070 & 0.345 & 0.263  \\
        \texttt{filewrong} (bug) & 4 & 45 & 0.241 & 0.051 & 0.189 & 0.086  \\
        \texttt{flow} & 4 & 16 & 0.078 & 0.028 & 0.049 & 0.028  \\
        \texttt{lock1} & 4 & 38 & 0.091 & 0.040 & 0.051 & 0.044  \\
        \texttt{lock2} & 4 & 45 & 0.407 & 0.047 & 0.360 & 0.221  \\
        \texttt{order5} & 5 & 52 & 0.431 & 0.059 & 0.372 & 0.222  \\
        \texttt{order5-2} & 5 & 40 & 0.299 & 0.050 & 0.249 & 0.149  \\
        \texttt{order5-variant} & 5 & 55 & 0.464 & 0.057 & 0.407 & 0.180  \\
        \texttt{twofiles} & 4 & 47 & 0.260 & 0.051 & 0.209 & 0.102  \\
        \texttt{twofilesexn} & 4 & 56 & 0.254 & 0.056 & 0.198 & 0.101  \\
\\
        \texttt{checknz} & 2 & 93 & 0.077 & 0.040 & 0.037 & 0.031  \\
        \texttt{checkpairs} (bug) & 2 & 251 & 0.243 & 0.059 & 0.184 & 0.073  \\
        \texttt{filepath} & 2 & 5956 & 0.365 & 0.153 & 0.212 & 0.206  \\
        \texttt{filter-nonzero} (bug) & 5 & 484 & 1.532 & 0.097 & 1.435 & 1.084  \\
        \texttt{filter-nonzero-1} & 5 & 890 & 5.129 & 0.163 & 4.966 & 4.038  \\
        \texttt{last} & 2 & 193 & 0.119 & 0.053 & 0.066 & 0.060  \\
        \texttt{map-head-filter} (bug) & 3 & 370 & 0.388 & 0.074 & 0.314 & 0.144  \\
        \texttt{map-head-filter-1} & 3 & 880 & 0.391 & 0.114 & 0.277 & 0.268  \\
        \texttt{map-plusone} & 5 & 302 & 0.868 & 0.096 & 0.772 & 0.620  \\
        \texttt{map-plusone-1} & 5 & 459 & 1.402 & 0.109 & 1.293 & 1.042  \\
        \texttt{map-plusone-2} & 5 & 704 & 2.762 & 0.134 & 2.628 & 1.822  \\
        \texttt{mkgroundterm} & 2 & 379 & 0.219 & 0.075 & 0.144 & 0.137  \\
        \texttt{risers} & 2 & 563 & 0.348 & 0.094 & 0.254 & 0.136  \\
        \texttt{safe-head} & 3 & 354 & 0.365 & 0.074 & 0.290 & 0.110  \\
        \texttt{safe-init} & 3 & 680 & 0.661 & 0.095 & 0.566 & 0.183  \\
        \texttt{safe-tail} & 3 & 468 & 0.493 & 0.089 & 0.404 & 0.144  \\
        \texttt{tails} & 3 & 259 & 0.147 & 0.064 & 0.083 & 0.077  \\
\\
        \texttt{g41} & 4 & 31 & --- & 0.039 & --- & 0.243  \\
        \texttt{merge4} & 2 & 141 & 0.516 & 0.254 & 0.262 & 0.175  \\
        \texttt{stress} & 1 & 35 & 0.058 & 0.028 & 0.029 & 0.023  \\
\\
        \texttt{cfa-life2} & 14 & 7648 & --- & 0.474 & --- & ---  \\
        \texttt{cfa-matrix-1} & 8 & 2944 & 18.098 & 0.323 & 17.775 & 17.768  \\
        \texttt{cfa-psdes} & 7 & 1819 & 1.798 & 0.262 & 1.536 & 1.528  \\
        \texttt{dna} & 2 & 411 & 7.062 & 0.177 & 6.885 & 6.415  \\
        \texttt{exp4-5} & 4 & 55 & --- & 0.048 & --- & 2.041  \\
        \texttt{fibstring} & 4 & 29 & --- & 0.042 & --- & 0.261  \\
        \texttt{filewrong} (bug) & 4 & 45 & 0.211 & 0.051 & 0.160 & 0.084  \\
        \texttt{fold\_fun\_list} & 7 & 1346 & 1.363 & 0.200 & 1.164 & 1.157  \\
        \texttt{fold\_right} & 5 & 1310 & 1.190 & 0.201 & 0.989 & 0.969  \\
        \texttt{jwig-cal\_main} & 2 & 7627 & 2.492 & 2.425 & 0.067 & 0.061  \\
        \texttt{l} & 3 & 35 & 0.256 & 0.043 & 0.213 & 0.204  \\
        \texttt{search-e-church} (bug) & 6 & 837 & 5.389 & 0.152 & 5.237 & 1.730  \\
        \texttt{specialize\_cps\_coerce1-c} & 3 & 2731 & 0.950 & 0.314 & 0.636 & 0.626  \\
        \texttt{tak} (dunno) & 8 & 451 & 57.130 & 0.134 & 56.997 & 45.523  \\
        \texttt{xhtmlf-div-2} (bug) & 2 & 3003 & 2.327 & 1.946 & 0.381 & 0.354  \\
        \texttt{xhtmlf-m-church} & 2 & 3027 & 2.394 & 2.040 & 0.354 & 0.345  \\
        \texttt{zip} & 4 & 2952 & 2.808 & 0.303 & 2.505 & 1.055  \\

        \bottomrule
    \end{tabular}
\end{center}
